# Supplementary material for: Linear-Time Self Attention with Codeword Histogram for Efficient Recommendation
Source: arXiv:2105.14068 source file (2021-05-28)
Supplement: Supplementary file 1 [file appendix.tex]

\appendix

\section{Appendix}
\subsection{LISA in Bidirectional Mode}
\label{app:lisa_bidirectional}

{
\removelatexerror
\begin{algorithm}[H]
\caption{LISA (bidirectional mode)}
\SetKwInOut{Input}{Input}
\SetKwInOut{Output}{Output}
\SetKwInOut{Parameters}{Parameters}
\label{alg:lisa_bidirectional}
\Input{Codeword indices of the sequence $\Psi \in \mathbb{N}^{L\times B}$}
\Parameters{Inner product table (after taking the exponent) $\mathbf{M} \in \mathbb{R}^{B\times W\times W}$, where $\mathbf{M}_{b,i,j}=\exp{\left((P^Q c^b_{i})^T (P^K c^b_{j})\right)}$; projected codebooks for values $\mathbf{C}^V=\mathbf{C}P^V \in \mathbb{R}^{B\times W \times D}$}
\Output{The results of self-attention $X' \in \mathbb{R}^{L\times D}$}
Convert $\Phi$ to one-hot representations $\mathbf{E}=\operatorname{one-hot}(\Phi) \in \{0,1\}^{L\times B\times W}$\;
Compute the sum $\mathbf{F}$ of $\mathbf{E}$ along the first dimension to get the codeword histogram of the whole sequence for each codebook\;
Gather inner product terms $\mathbf{S} \in \mathbb{R}^{L\times B \times W}$ from $\mathbf{M}$ along the first two dimensions using indices $\Phi$\;
$\mathbf{A} = \mathbf{F} \otimes \mathbf{S}$ (element-wise multiplication, broadcast $\mathbf{F}$)\;
Normalize the attention scores $A$ along the last dimension\;
$X'= \sum_{b=1}^B \mathbf{A}_{:,b,:}\mathbf{C}^V_{b,:,:}$\;
\Return X'
\end{algorithm}
}
